# Supplementary material for: Accelerating the Search for Superconductors Using Machine Learning
Source: arXiv:2505.11964 source file (2025-12-16)
Supplement: Supplementary file 1 [file Supplementary_Information.pdf]

# Supplementary Information for Accelerating the Search for Superconductors Using Machine Learning

Suhas Adiga[1,2] and Umesh V. Waghmare[1]

[1] *Theoretical Sciences Unit, School of Advanced Materials (SAMat), Jawaharlal Nehru Centre for Advanced Scientific Research, Jakkur, Bengaluru 560064, India*

[2] *Chemistry and Physics of Materials Unit, Jawaharlal Nehru Centre for Advanced Scientific Research, Jakkur, Bengaluru 560064, India*

(Dated: May 14, 2025)

## I. QUANTUM STRUCTURAL DIAGRAM PARAMETERS

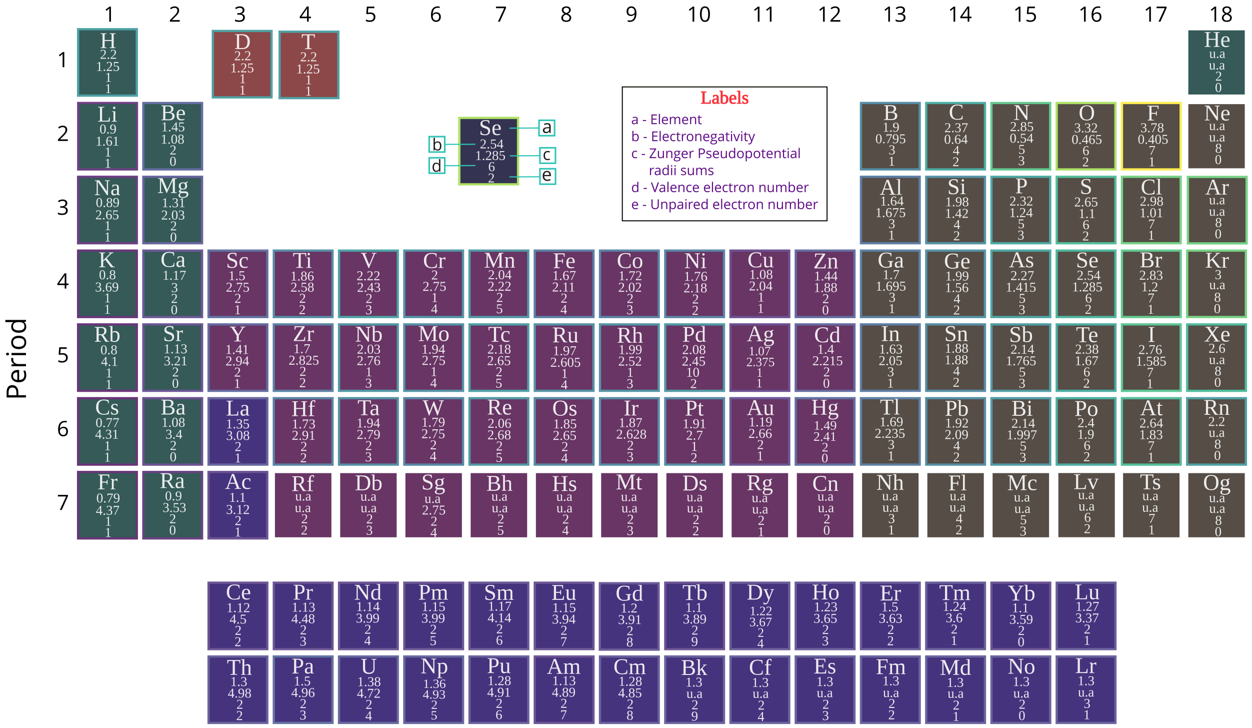


u.a- Data Unavailable

FIG. S1. Periodic table with elemental parameters used for feature generation.

To calculate descriptors from Quantum Structure Diagrams [1] and engineered features, we require the values of electronegativity on the Martynov-Batsanov scale, the sum of Zunger pseudopotential radii, the number of valence electrons, and the number of unpaired electrons. We obtain the electronegativity values on the Martynov-Batsanov scale and the sums of Zunger pseudopotential radii from [2]. For elements with no reported electronegativity on the Martynov-Batsanov scale, we approximate them using the Pauling scale, as the Martynov-Batsanov electronegativity is the square root of the average valence ionization energy, and both scales have the same dimension of $(eV)^{\frac{1}{2}}$.

For compounds containing curium (Cm), which appear frequently in the dataset, we approximate the Zunger pseudopotential radii sum using the formula:

$$R_{\mathrm{Cm}} = \left(\frac{R_{\mathrm{Am}}}{R_{\mathrm{Eu}}}\right) \times R_{\mathrm{Gd}} \tag{1}$$

Fig. S1 displays a periodic table with the parameter values used for feature generation.

## II. MACHINE LEARNING MODELS

We classify compounds as superconductors or non-superconductors following the approach outlined in Sec III B of our manuscript. To benchmark the performance of classification model, we identify the best-performing model for this task. Specifically, we select the top five models based on their training and test metrics and rank them by test accuracy, as presented in Table S1. An accuracy of 1 indicates perfect classification, meaning no misclassifications (both false positives and false negatives), which we aim to minimize. All machine learning tasks here are implemented using the *scikit-learn* [3] package in Python.

$$\text{Accuracy} = \frac{\text{TP} + \text{TN}}{\text{TP} + \text{TN} + \text{FP} + \text{FN}}$$

$$\text{Recall} = \frac{\text{TP}}{\text{TP} + \text{FN}}$$

$$\text{Precision} = \frac{\text{TP}}{\text{TP} + \text{FP}}$$

$$\text{F1 Score} = 2 \times \frac{\text{Precision} \times \text{Recall}}{\text{Precision} + \text{Recall}}$$

where TP, TN, FP and FN stands for True Positive, True Negative, False Positive and False negative respectively.

| Model | Training Metrics | | | | Testing Metrics | | | |
|---|---|---|---|---|---|---|---|---|
| | Accuracy | Recall | Precision | F1 Score | Accuracy | Recall | Precision | F1 Score |
| Random Forest | 0.990 | 0.990 | 0.990 | 0.990 | 0.934 | 0.983 | 0.945 | 0.964 |
| Extra Trees | 1.000 | 1.000 | 1.000 | 1.000 | 0.929 | 0.976 | 0.947 | 0.961 |
| XGBoost | 0.985 | 0.998 | 0.985 | 0.992 | 0.932 | 0.981 | 0.945 | 0.963 |
| Catboost | 0.951 | 0.998 | 0.949 | 0.973 | 0.932 | 0.991 | 0.936 | 0.963 |
| KNN | 0.931 | 0.985 | 0.939 | 0.962 | 0.920 | 0.979 | 0.936 | 0.957 |

TABLE S1. Benchmark Metrics for Classification on *SuperCon-MTG* Database using an 80-20 Train-Test Split (with Default Model Parameters)

Random Forest [4] is an ensemble learning method that constructs multiple decision trees using bagging. Specifically, it selects random samples with replacement (bootstrapping) from the dataset to train each tree. This means that after a sample is drawn from the dataset, it is returned to the bag, making it possible for the same sample to be selected multiple times for training different trees. For regression tasks, the final output is the average prediction of individual trees, whereas for classification, it is determined by majority voting. This random sampling process helps reduce overfitting and variance.
In contrast, Extra Trees [5], another ensemble method, trains each tree on the entire dataset rather than using bootstrapped samples. This often leads to overfitting, as reflected in the training metrics, where the model appears to have memorized the data. Meanwhile, XGBoost [6] demonstrates stable performance on the test dataset. However, we choose Random Forest over XGBoost due to its robustness to noise, stemming from its randomized sampling of both datapoints and features. Additionally, Random Forest achieves slightly better test metrics than XGBoost in classification.
Using the Random Forest classification model, we predict superconductors in both the training and test datasets. The predicted superconductors from the training dataset is then used for training the machine learning model to predict critical temperature. We evaluate the top five performing models based on their training and test metrics, as presented in Table S2.

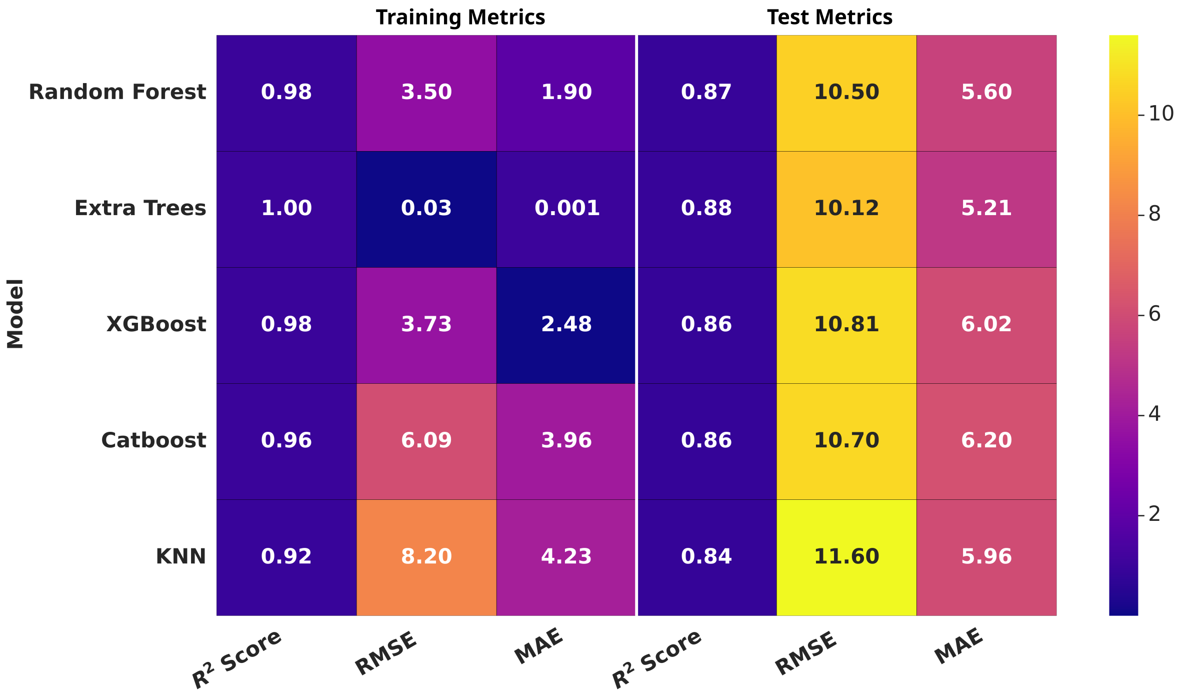


TABLE S2. Benchmark Metrics for Regression models on Superconductors classified using Random Forest classification model (with Default Model Parameters)

The Random Forest model demonstrates higher performance on both training and test data, achieving the highest $R^2$ score and the lowest root mean squared error (RMSE) and mean absolute error (MAE), thereby outperforming other models in critical temperature prediction. In contrast, the Extra Trees regressor exhibits overfitting, as evident in its training metrics, where it memorizes the data. Given its superior generalization ability, we choose the Random Forest model for both classification and regression tasks.

$$R^2 \text{ Score} = 1 - \frac{\sum_{i=1}^{n} \left[(T_c)_i - (T_c)_{\text{predicted},i}\right]^2}{\sum_{i=1}^{n} \left[(T_c)_i - \overline{T_c}\right]^2}$$

$$\text{RMSE} = \sqrt{\frac{\sum_{i=1}^{n} \left[(T_c)_i - (T_c)_{\text{predicted},i}\right]^2}{n}}$$

$$\text{MAE} = \frac{1}{n}\sum_{i=1}^{n} \left|(T_c)_i - (T_c)_{\text{predicted},i}\right|$$

where $T_c$ is the experimental critical temperature, $(T_c)_{predicted}$ is critical temperature predicted using machine learning and $\overline{T_c}$ is the mean critical temperature of 'n' samples in the datapoints

## III. HYPERPARAMETER TUNING

### A. Bayesian Optimization for Classification

Bayesian optimization was performed for 400 iterations to determine optimal hyperparameters for the Random Forest classification model. The best parameters identified are:

- `n_estimators` = 500
- `max_depth` = 94
- `max_features` = 0.9
- `min_samples_leaf` = 2
- `min_samples_split` = 2

In a random forest model, `n_estimators` represents the number of trees in the forest, `max_depth` is the maximum depth of each tree, `max_features` defines the maximum proportion of features considered at each split, `min_samples_leaf` specifies the minimum number of samples required in each leaf node, and `min_samples_split` is the minimum number of samples required to split an internal node.

### B. Bayesian Optimization for Regression

For the Random Forest regression model, Bayesian optimization also used 400 iterations, yielding:

- `n_estimators` = 175
- `max_depth` = 38
- `max_features` = 0.52
- `min_samples_leaf` = 2
- `min_samples_split` = 2

### C. Bayesian Optimization for Regression for 5-Key Feature mode

Using only 5 features identified via SHAP analysis, regression hyperparameters optimized through Bayesian search:

- `n_estimators` = 336
- `max_depth` = 53
- `max_features` = 0.71
- `min_samples_leaf` = 2
- `min_samples_split` = 2

## IV. DATA ANALYTICS OF COMPOUNDS BY CLASS

The Table S3 presents the class, count, average critical temperature, and maximum critical temperature of 12,384 compounds from SuperCon-MTG, as classified by our Random Forest Classification Model

TABLE S3. Statistics of compounds classified as superconductors from SuperCon-MTG by class.

| Class | Count | Avg $T_c$ (K) | Max $T_c$ (K) |
|---|---|---|---|
| Alloys | 2653 | 4.9 | 29.8 |
| Bi-based | 216 | 9.6 | 31.5 |
| Borides | 457 | 12.8 | 41.4 |
| Borocarbides | 286 | 10.8 | 38.5 |
| Carbon-based | 205 | 9.3 | 33.0 |
| Cuprates | 4193 | 53.1 | 143 |
| Germanides | 297 | 6.5 | 21.0 |
| Heavy Fermions | 545 | 2.6 | 16.6 |
| Iron Chalcogenides | 679 | 22.0 | 56.5 |
| Iron Pnictides | 578 | 18.6 | 54.0 |
| Nitrides | 170 | 12.1 | 26.0 |
| Oxides | 252 | 5.2 | 57.5 |
| Silicides | 444 | 5.7 | 19.2 |
| Tellurides | 258 | 2.3 | 8.6 |
| Transition Metal Pnictides | 172 | 4.7 | 19.2 |
| Others | 979 | 5.2 | 37.8 |

## V. COMPOSITION GENERATION USING BINARY ELEMENTAL COMBINATIONS

To explore chemically viable regions of the compositional space, we generate binary compositions using one transition metal (in Figure S2) and one main group (in Figure S3) element. Radioactive or unstable elements such as Tc, Po, and At are excluded.

Each generated composition is passed through the SMACT [7] filter to ensure:

- Charge neutrality,
- Electronegativity ordering (cation less than anion),
- Valid oxidation state pairings.

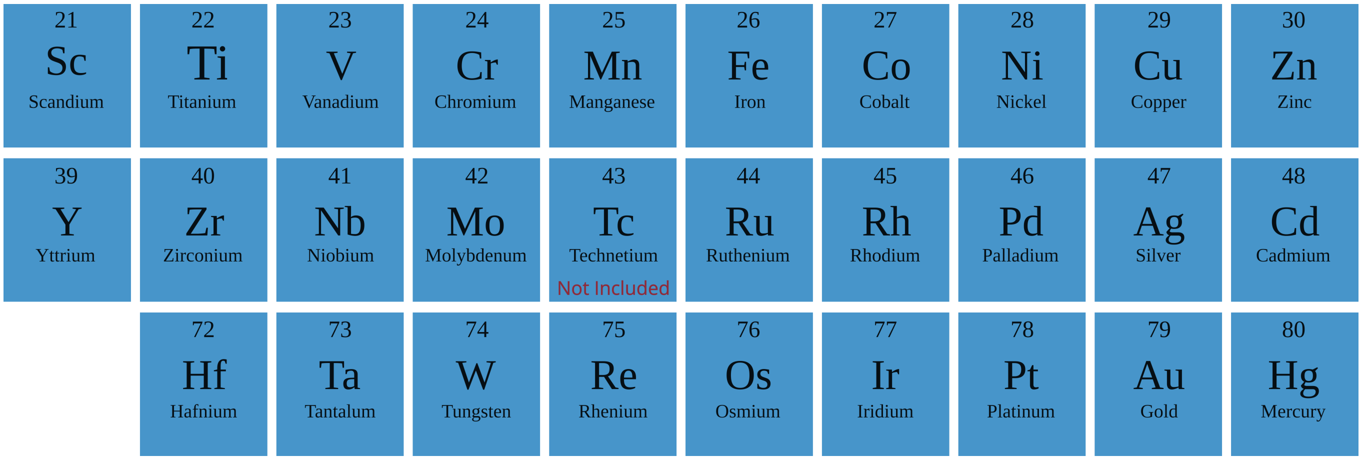


FIG. S2. Transition metals used for binary composition generation. Technetium (Tc) excluded.

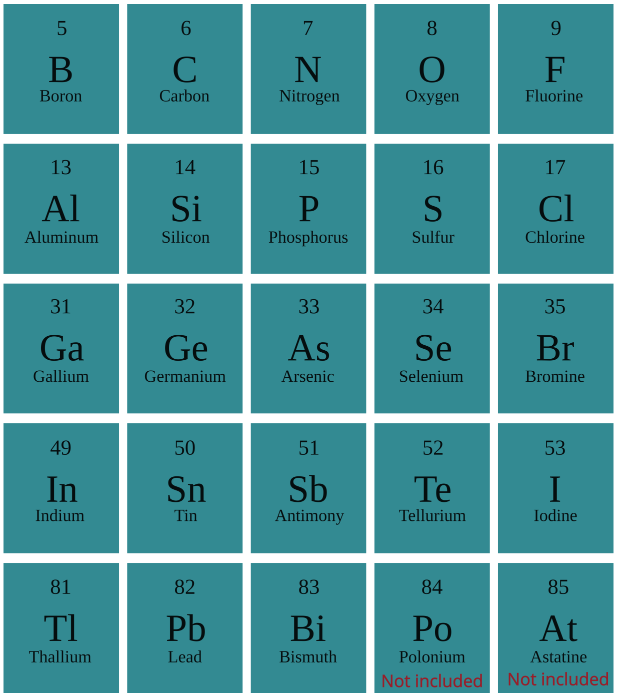


FIG. S3. Main group elements used for binary composition generation. Po and At excluded.

## VI. SMACT PROBABILITY CALCULATION FOR GENERATED COMPOSITIONS

SMACT ensures chemical feasibility by checking charge neutrality and oxidation state compatibility. For a compound $A_mB_nX_p$ with oxidation states $a$, $b$, and $c$, the formation probability is given by:

$$P_{A_mB_nX_p} = \frac{N_{AX}}{N_{M_AX}} \times \frac{N_{BX}}{N_{M_BX}}$$

where:

- $N_{AX}$: Number of times element $A$ with oxidation state $a$ occurs with anion $X$.
- $N_{M_AX}$: Total occurrences of $A$ with $X$ across all oxidation states.
- $N_{BX}$ and $N_{M_BX}$: Similarly for element $B$.
- $X$: Most electronegative element among $A$, $B$, and $X$.

Data used for this calculation is derived from the ICSD via the Materials Project.
**Note:** If a combination is not found:

```
NameError: One or both of [Mg2, H-1] are not in the probability table.
```

This error indicates insufficient data for calculating a valid probability for that specific oxidation state pair.

[1] J. C. Phillips, Quantum structural diagrams, in *Electronic Materials* (Springer Berlin Heidelberg, 1991) p. 287–306.
[2] P. Villars and F. Hulliger, Journal of the Less Common Metals **132**, 289–315 (1987).
[3] F. Pedregosa, G. Varoquaux, A. Gramfort, V. Michel, B. Thirion, O. Grisel, M. Blondel, P. Prettenhofer, R. Weiss, V. Dubourg, J. Vanderplas, A. Passos, D. Cournapeau, M. Brucher, M. Perrot, and Édouard Duchesnay, Journal of Machine Learning Research **12**, 2825 (2011).

[4] L. Breiman, Machine Learning **45**, 5 (2001).
[5] P. Geurts, D. Ernst, and L. Wehenkel, Machine Learning **63**, 3–42 (2006).
[6] T. Chen and C. Guestrin, in *Proceedings of the 22nd ACM SIGKDD International Conference on Knowledge Discovery and Data Mining*, KDD '16 (ACM, 2016) p. 785–794.
[7] D. Davies, K. Butler, A. Jackson, J. Skelton, K. Morita, and A. Walsh, Journal of Open Source Software **4**, 1361 (2019).
